# Supplementary material for: From Coarse to Fine-grained Concept based Discrimination for Phrase Detection
Source: arXiv:2112.03237 source file (2022-11-15)
Supplement: Supplementary file 1 [file 8_supp_mod.tex]

\section{BISON benchmark}
\label{sec:image-sentence-supp}
In Section \ref{sec:related} of our paper we used the BISON benchmark \cite{Hu2019BinaryIS} to demonstrate how good performance on phrase detection leads to improved downstream task performance (unlike the localization-only task evaluated in most prior work).  In this benchmark, the model is asked to select the caption that best fits an image from a pair of semantically similar images.  Formally, given input image $I$ and and a set of noun phrases representing a the caption $S$, we would use a scoring function (\ie, a phrase grounding method) to measure the relationship between each phrase $S_{p_i}$, \ie, $\text{PhraseScore}(S_{p_i}, I)$.  Then, we compute the Image-Caption score $\text{ImgScore}(S, I)$ as follows: 

\begin{equation}
  \text{ImgScore}(S, I) = \frac{1}{|S|} \sum_{i=0}^{|S|} \text{PhraseScore}(S_{p_{i}}, I)
  \label{eq:image-sentence}
\end{equation}

\noindent We rank images for a given caption using Eq.~(\ref{eq:image-sentence}), then select the image with the bigger score.

 \begin{table*}[t!]%{\textwidth}
    \setlength{\tabcolsep}{3pt}
        \centering
        \begin{tabular}{rlcccccccc}
        \toprule
         &  & \multicolumn{4}{c}{Flickr30K Entities} & \multicolumn{4}{c}{RefCOCO+} \\ \midrule
         &  & zero- & few- & \multicolumn{1}{c}{com-} &  & zero- & few- & \multicolumn{1}{c}{com-} &  \\
         & \#Train Samples & shot & shot & \multicolumn{1}{c}{mon} & mean & shot & shot & \multicolumn{1}{c}{mon} & mean \\ \midrule
        \multicolumn{1}{l}{} & MDETR \cite{Kamath_2021_ICCV} & 1.6 & 2.6 & \multicolumn{1}{c}{8.0} & 4.0 & 1.4 & 2.8 & \multicolumn{1}{c}{11.0} & 5.0 \\
        \multicolumn{1}{l}{} & GLIP \cite{li2021grounded} & 4.3 & 6.8 & \multicolumn{1}{c}{13.7} & 8.3 & 1.9 & 4.4 & \multicolumn{1}{c}{12.6} & 6.3 \\
        \multicolumn{1}{l}{} & CCA \cite{Plummer_2020} & 8.9 & 10.7 & \multicolumn{1}{c}{18.9} & 12.9 & 5.7 & 8.3 & \multicolumn{1}{c}{20.9} & 11.7 \\
         & SimNet w/CCA \cite{Plummer_2020} & 9.4 & 11.2 & \multicolumn{1}{c}{19.8} & 13.5 & 6.2 & 10.3 & \multicolumn{1}{c}{20.5} & 12.3 \\ \midrule
         & +NCC & 10.6 & 12.1 & \multicolumn{1}{c}{20.4} & 14.3 & 6.2 & 10.3 & \multicolumn{1}{c}{21.8} & 12.8 \\
         & +NPA & 10.3 & 12.4 & \multicolumn{1}{c}{20.8} & 14.5 & 5.9 & 10.5 & \multicolumn{1}{c}{23.6} & 13.3 \\
         & +NPA+NCC & 10.7 & 12.7 & \multicolumn{1}{c}{21.4} & 15.0 & 6.4 & 10.5 & \multicolumn{1}{c}{23.8} & 13.5 \\
         & CFCD-Net (+ NPA + NCC + FGM) & \textbf{11.0} & \textbf{13.4} & \multicolumn{1}{c}{\textbf{21.7}} & \textbf{15.4} & \textbf{6.5} & \textbf{10.5} & \multicolumn{1}{c}{\textbf{24.2}} & \textbf{13.8} \\ \bottomrule
        \end{tabular}
     \caption{ mAP split by frequency of training instances where  \textbf{augmented positive phrases (PPA)} from \cite{Plummer_2020} is used for evaluation. The table compares our model three components (NPA, NCC, and FGM) to state of the art (SimNet w/CCA). See Section \ref{sec:results_discussion} for discussion}
    \label{tb:main_results_ppa}
\end{table*}

\begin{table}[t!]
    \setlength{\tabcolsep}{2pt}
    \centering
    \caption{Phrase Localization accuracy of prior work SimNet w/CCA and our model three components: NPA, NCC, FGM. Section~\ref{phrase-loc-supp} for discussion.}
    \begin{tabular}{lcc}
    \toprule
     & \begin{tabular}[c]{@{}c@{}}Flickr30K \\ Entities\end{tabular} & \begin{tabular}[c]{@{}c@{}}Ref\\ COCO+\end{tabular} \\ \midrule
    SimNet w/CCA & 71.9 & 57.5 \\
    +NPA & 70.6 & 56.3 \\
    +NPA+CR & 70.3 & 55.9 \\
    PFP-Net(+NPA+CR+FGM) & 70.3 & 55.9 \\ \bottomrule
    \end{tabular}   
    \label{loc_no_ppa}
     \vspace{-2mm}
\end{table}

\section{Positive Phrase Augmentation (PPA)}
\label{ppa-supp}

Table \ref{tb:main_results_ppa} reports the performance of CFCD-Net using positive phrase augmentation (PPA) \cite{Plummer_2020}, which reduces annotation sparsity by pairing ground truth phrases with plausible positive phrases using WordNet \cite{10.1145/219717.219748}. We note that PPA does not change the relative gains of the detection methods, but obtains higher absolute performance.

\section{Phrase localization performance}
\label{phrase-loc-supp}

As discussed in Section \ref{sec:related}, we note that localization and detection performance are not causally related. However, to be complete, we report localization performance of our model in Table~\ref{loc_no_ppa}. We note that our methods' localization numbers are on par with previous work.

\begin{table}[t!]
    \caption{\textbf{Dataset annotations' false negative rate.} See Section~\ref{supp_datasets} for more details.}

    \setlength{\tabcolsep}{2pt}
    \centering
    \begin{tabular}{lc}
    \toprule
     & False \\ 
     & Negative\% \\ 
     \midrule
    Referit \cite{KazemzadehOrdonezMattenBergEMNLP14} & 74\% \\
    Visual Genome \cite{krishnavisualgenome} & 72\% \\
    Flickr30k Entities \cite{7410660} & 31\% \\
    RefCOCO+  \cite{10.1007/978-3-319-46475-6_5}& 40\% \\ \bottomrule
    \end{tabular} 

    \vspace{-1mm}
    \label{false_neg}
\end{table}

\section{Evaluation dataset selection}
\label{supp_datasets}

The sparsity of phrase detection datasets annotations poses significant challenges on evaluation. Real world datasets annotations can not cover all the possible positive cases. For example, a region annotated with only the phrase \textit{blue shirt} can also be correctly labeled with \textit{clothing}. \citet{Plummer_2020} attempted to mitigate this problem by introducing Positive Phrase Augmentations (PPA) where structures like WordNet \cite{10.1145/219717.219748} were used to derive additional positive samples. However, this problem is not limited to issues with synonyms. Phrases might have different structures but can convey the same meaning (\eg frisbee that is round vs a round frisbee), While the authors of Flickr30K \cite{7410660} limited the structure of their annotations to mitigate this problem, this is not the case for datasets like Visual Genome \cite{krishnavisualgenome} or Referit \cite{KazemzadehOrdonezMattenBergEMNLP14} therefore, their validity for phrase detection evaluation is not clear. To quantitatively document this issue, we sampled 30 random phrases from each dataset and considered the top 5 most similar phrases using the visual based language representation ViCo \cite{gupta2019vico}. For each of these top 5 phrases, we manually counted the number of false negatives. We report the average results in Table~\ref{false_neg}. Note that both Referit and Visual Genome suffer from significantly higher false negative rates than Flickr30k Entities. Thus, they are not viable evaluation datasets for phrase detection. We instead use Flickr30k Entities and  RefCOCO+ \cite{10.1007/978-3-319-46475-6_5} which was collected using the same underlying game as Referit but  with improved data collection standards. Thus the phrases were more appearance focused and concise as evident in the lower false negative rate Table~\ref{false_neg}.
